# Supplementary material for: MobiEdit: Resource-efficient Knowledge Editing for Personalized On-device LLMs
Source: arXiv:2506.13772 source file (2025-06-05)
Supplement: Supplementary file 1 [file appendix.tex]

\appendix
\section{Evaluation on Llama3.2-3B-Instruct}
\sys demonstrates superior performance and editing quality on the Llama3.2-3B-Instruct architecture.
As shown in Table~\ref{tab:table_llama3.2_zsre_perf}, \sys (MobiEdit) requires only 5 GB of memory, while baseline methods consume 34 GB.
On average, \sys achieves a 3.09$\times$ latency improvement compared to ROME, MEMIT, and AlphaEdit, and a 6.19$\times$ improvement over WISE.
For energy efficiency, \sys provides a 12.43–28.68$\times$ improvement.
Our method attains an edit success score of 88.3, as shown in Table~\ref{tab:table_llama3.2_zsre_edit}, despite minor accuracy degradation caused by prefix cache and weight quantization.

Compared to Qwen2.5-3B-Instruct’s average latency of 1530 seconds, Llama3.2-3B-Instruct with \sys achieves a lower latency of 1411 seconds on average.
This efficiency is attributed to the NPU-friendly design of Llama3.2-3B-Instruct, which features a hidden size of 3072 and 28 layers—compared to Qwen2.5-3B’s configuration of 2048 hidden dimensions and 36 layers.
The wider and shallower architecture (3072×28 vs. 2048×36) is more computationally favorable for NPUs.

\begin{table}[ht]
\caption{Comparison of our method with NPU and other knowledge editing methods with CPU on Llama3.2-3B-Instruct.}
\centering
\scriptsize
\setlength{\tabcolsep}{3pt}

\begin{subtable}[t]{\linewidth}
\caption{Performance Comparison}
\begin{tabular}{l c cc cc cc}
\toprule
\multirow{2}{*}{\textbf{Method}} & \multirow{2}{*}{\textbf{Memory (GB)}} 
& \multicolumn{2}{c}{\textbf{K60}} 
& \multicolumn{2}{c}{\textbf{K70}} 
& \multicolumn{2}{c}{\textbf{OnePlus}} \\
& & Time (s) & Energy (J) & Time (s) & Energy (J) & Time (s) & Energy (J) \\
\midrule
ROME & \cellbar{34.14}{0.75} & \cellbar{4834.78}{0.36} & \cellbar{0.27}{0.38} & \cellbar{4578.66}{0.50} & \cellbar{0.25}{0.47} & \cellbar{3551.82 }{0.50} & \cellbar{0.20}{0.47} \\
MEMIT & \cellbar{34.14}{0.75} & \cellbar{4834.78}{0.36} & \cellbar{0.27}{0.38} & \cellbar{4578.66}{0.50} & \cellbar{0.25}{0.47} & \cellbar{3551.82}{0.50} & \cellbar{0.20}{0.47} \\
WISE & \cellbar{35.05}{0.77} & \cellbar{9668.86 }{0.90} & \cellbar{0.53}{1.00} & \cellbar{9157.32}{1.00} & \cellbar{0.50}{1.00} & \cellbar{6505.63}{1.00} & \cellbar{0.39}{1.00} \\
AhphaEdit & \cellbar{34.14}{0.75} & \cellbar{4834.78}{0.36} & \cellbar{0.27}{0.38} & \cellbar{4578.66}{0.50} & \cellbar{0.25}{0.47} & \cellbar{3551.82}{0.50} & \cellbar{0.20}{0.47} \\
\textbf{MobiEdit} & \cellbargreen{5.06}{0.10} & \cellbargreen{1754.26}{0.10} & \cellbargreen{0.021}{0.04} & \cellbargreen{1362.26}{0.08} & \cellbargreen{0.017}{0.02} & \cellbargreen{1117.19}{0.08} & \cellbargreen{0.014}{0.02} \\
\bottomrule
\end{tabular}
\label{tab:table_llama3.2_zsre_perf}
\end{subtable}
\begin{subtable}[t]{\linewidth}
    \centering
    \caption{Edit Quality Comparison on ZsRE}
    % \resizebox{0.5\textwidth}{!}{
    \begin{tabular}{l|c|c|c|c}
    \hline
    & \textbf{ROME} & \textbf{zo} & \textbf{zo+prefix} & \textbf{zo+prefix+quan} \\
    \hline
    Edit Succ & 96.2 & 95.8 & 90.4 & 88.3 \\
    Portability & 51.3 & 50.6 & 44.2 & 38.3 \\
    Locality & 57.9 & 61.6 & 56.2 & 44.3 \\
    Fluency & 555 & 580 & 566 & 582 \\
    \hline
    \end{tabular}
    \label{tab:table_llama3.2_zsre_edit}
% \caption{CounterFact Dataset}
% \begin{tabular}{l c cc cc cc}
% \toprule
% \multirow{2}{*}{\textbf{Method}} & \multirow{2}{*}{\textbf{Memory (GB)}}
% & \multicolumn{2}{c}{\textbf{K60}} 
% & \multicolumn{2}{c}{\textbf{K70}} 
% & \multicolumn{2}{c}{\textbf{OnePlus}} \\
% & & Time (s) & Energy (J) & Time (s) & Energy (J) & Time (s) & Energy (J) \\
% \midrule
% ROME & \cellbar{46.14}{0.74} & \cellbar{4416.66}{0.23} & \cellbar{0.24}{0.36} & \cellbar{4156.86}{0.25} & \cellbar{0.23}{0.46} & \cellbar{3161.82}{0.26} & \cellbar{0.17}{0.45} \\
% MEMIT & \cellbar{46.14}{0.74} & \cellbar{4416.66}{0.23} & \cellbar{0.24}{0.36} & \cellbar{4156.86}{0.25} & \cellbar{0.23}{0.46} & \cellbar{3161.82}{0.26} & \cellbar{0.17}{0.45} \\
% WISE & \cellbar{46.30}{0.77} & \cellbar{11041.65}{1.00} & \cellbar{0.61}{1.00} & \cellbar{8313.72}{1.00} & \cellbar{0.46}{1.00} & \cellbar{6323.63}{1.00} & \cellbar{0.35}{1.00} \\
% AhphaEdit & \cellbar{46.14}{0.74} & \cellbar{4416.66}{0.23} & \cellbar{0.24}{0.36} & \cellbar{4156.86}{0.25} & \cellbar{0.23}{0.46} & \cellbar{3161.82}{0.26} & \cellbar{0.17}{0.45} \\
% \textbf{MobiEdit} & \cellbargreen{5.60}{0.10} & \cellbargreen{2105.12}{0.10} & \cellbargreen{0.026}{0.04} & \cellbargreen{1634.72}{0.08} & \cellbargreen{0.020}{0.02} & \cellbargreen{1340.63}{0.08} & \cellbargreen{0.016}{0.02} \\
% \bottomrule
% \end{tabular}
% \label{tab:table_llama3.2_zsre}
\end{subtable}
\label{tab:table_llama_performance}
\end{table}

\section{Loss Curve}
\begin{figure}[htbp]
    \centering
    
    % 子图1
    \begin{subfigure}[b]{0.32\textwidth}
        \centering
        \includegraphics[width=\textwidth]{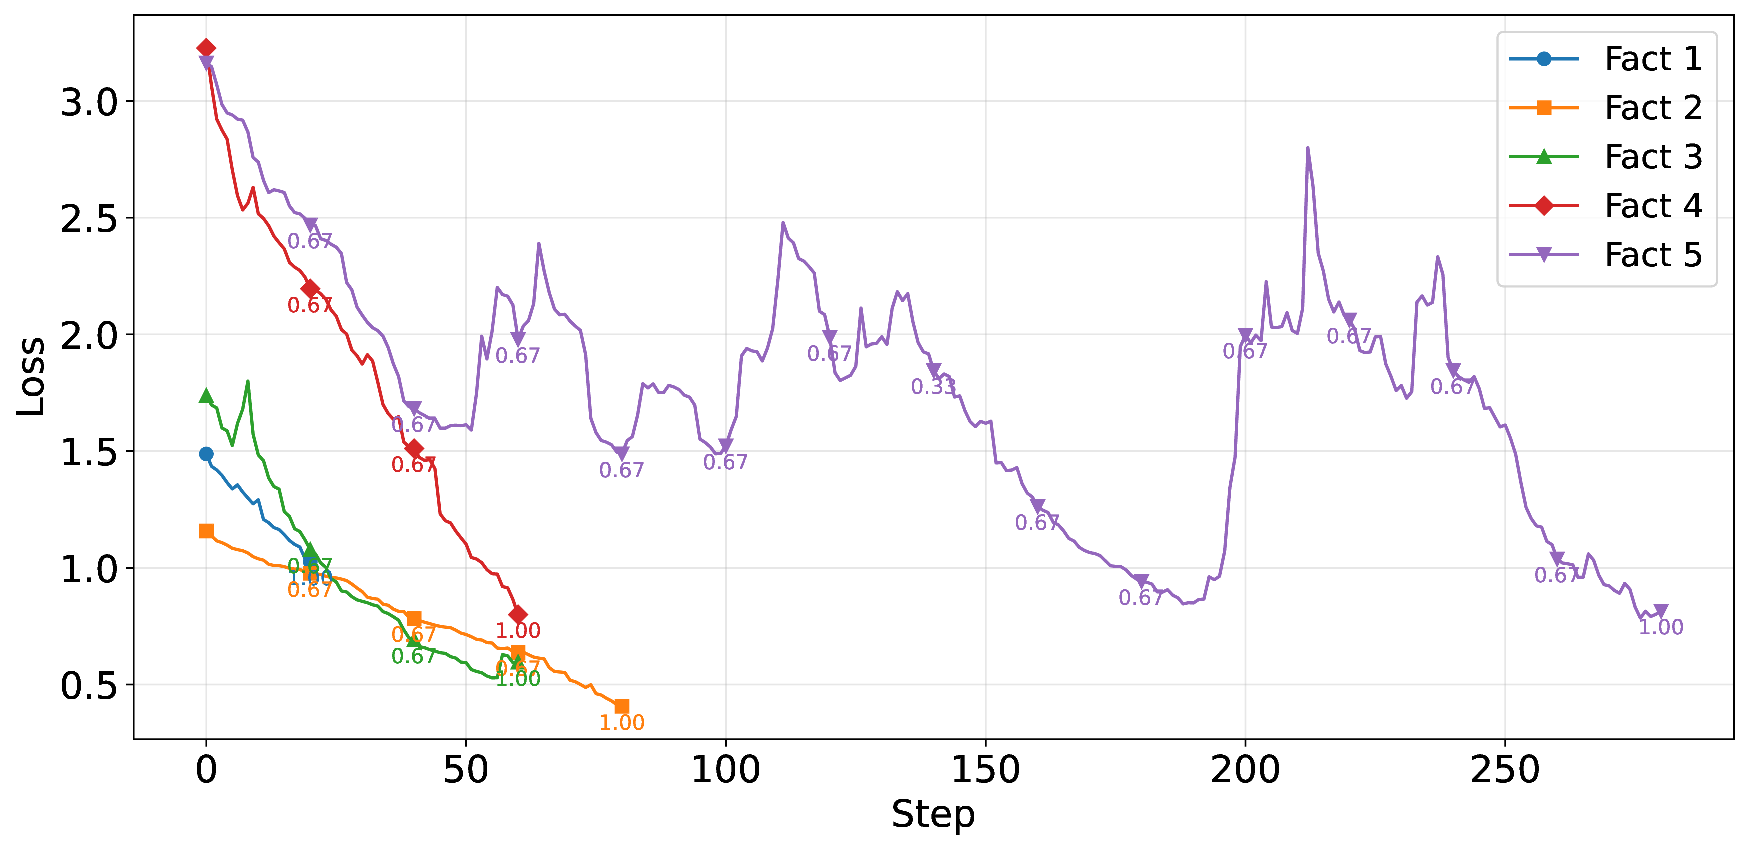}
        \caption{zo}
        \label{fig:loss_curve_zo}
    \end{subfigure}
    \hfill
    % 子图2
    \begin{subfigure}[b]{0.32\textwidth}
        \centering
        \includegraphics[width=\textwidth]{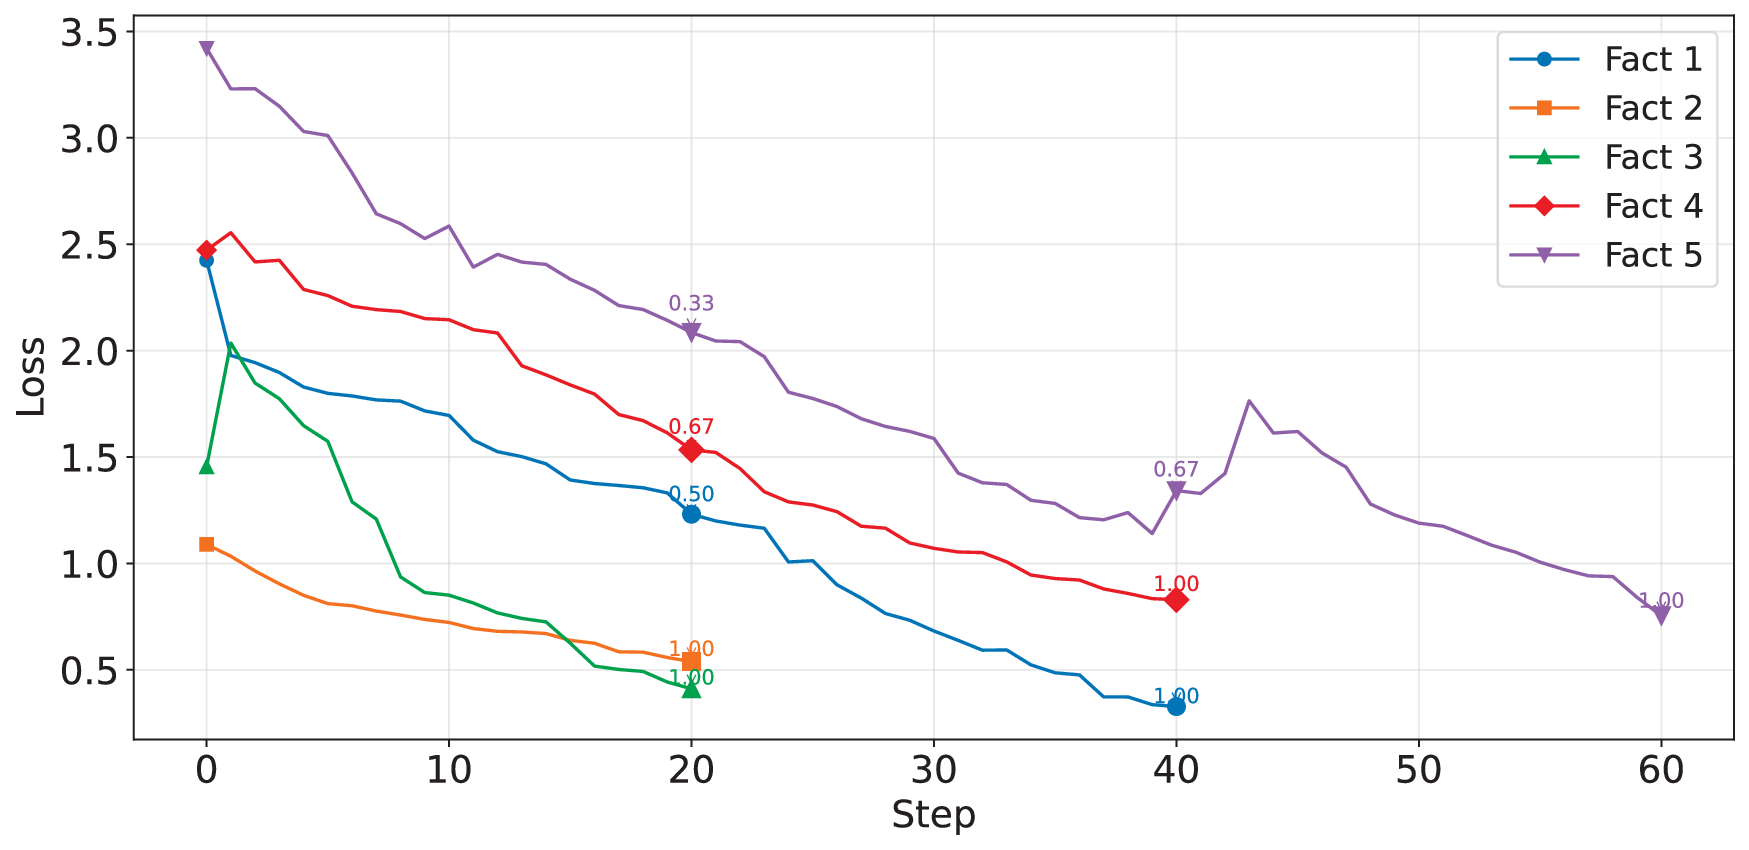}
        \caption{zo + prefix}
        \label{fig:loss_curve_zo_prefix}
    \end{subfigure}
    \hfill
    % 子图3
    \begin{subfigure}[b]{0.32\textwidth}
        \centering
        \includegraphics[width=\textwidth]{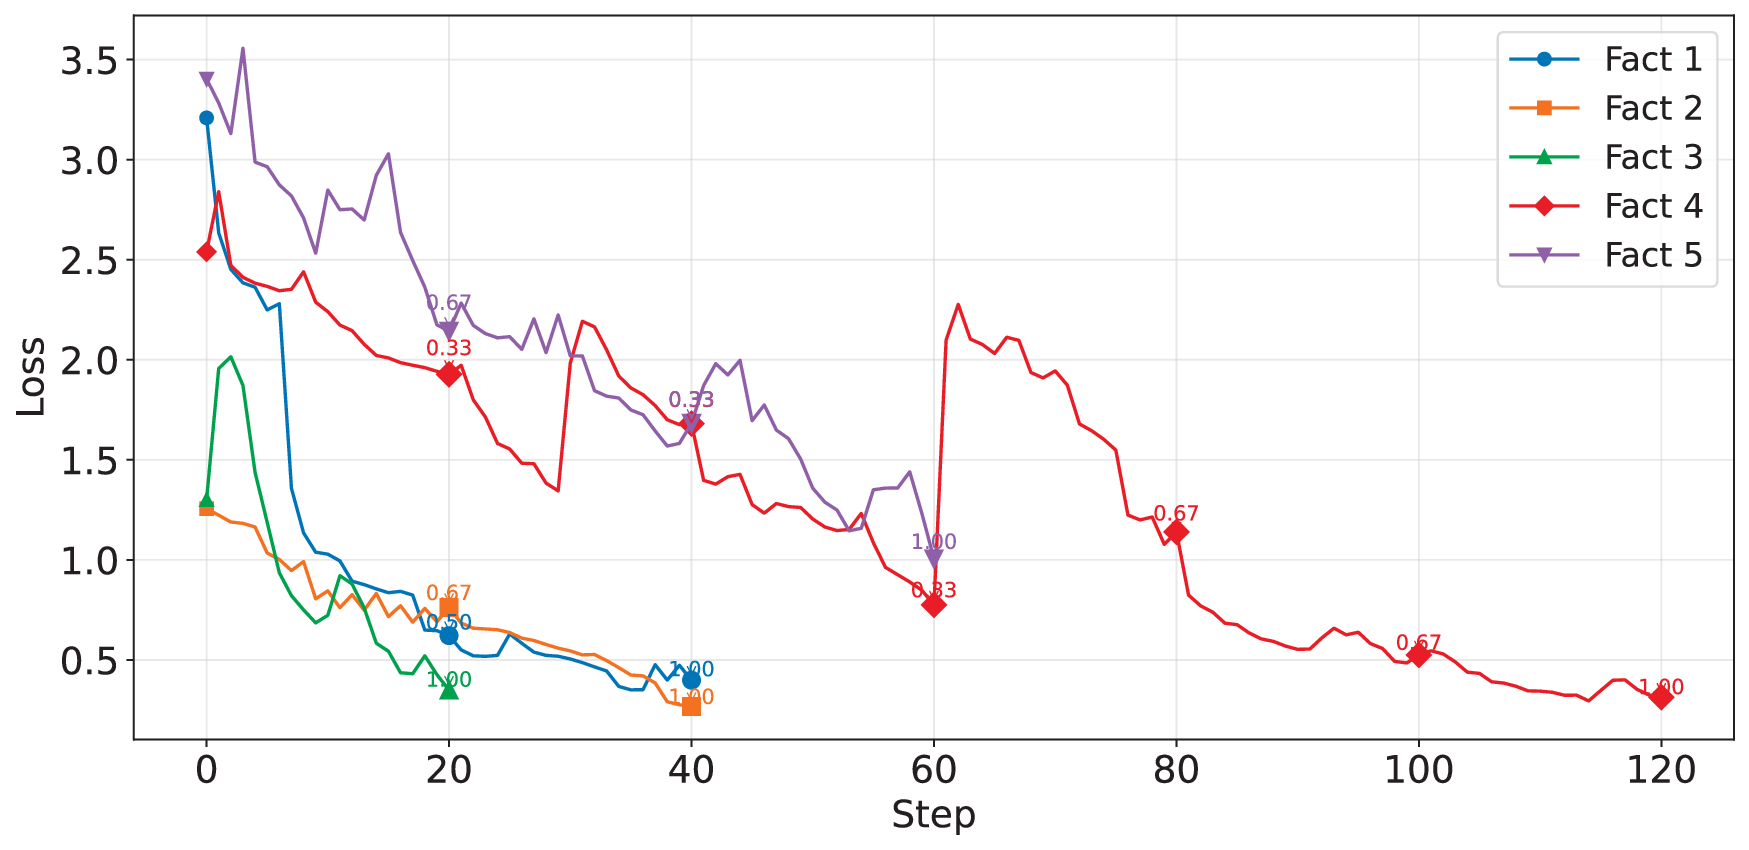}
        \caption{zo + prefix + quan}
        \label{fig:loss_curve_zo_prefix_quan}
    \end{subfigure}
    
    \caption{Loss curve of Llama3.2 with ZsRE }
    \label{fig:loss_curve}
\end{figure}
We illustrate the loss curves under three configurations: ZO, ZO+Prefix Cache, and ZO+Prefix Cache+Quantization in Figure~\ref{fig:loss_curve}. Using an early stopping controller, all knowledge edits terminated immediately upon successful editing. Notably, prefix cache demonstrated remarkable optimization acceleration - Fact 5 exhibited a 5$\times$ reduction in required training steps (from 300 to 60 steps). Although quantization introduced transient oscillations during gradient descent, it maintained final convergence accuracy, albeit with increased optimization time, as demonstrated by Fact 4’s step count rising from 40 to 120.

\section{Hyperparameters}
\begin{figure}[htbp]
    \centering
    
    \begin{subfigure}[b]{0.24\textwidth}
        \centering
        \includegraphics[width=\textwidth]{figs/test_v1_eval_lr5e-1_4_loss_curve.pdf}
        \caption{1 direction}
        \label{fig:v1}
    \end{subfigure}
    \hfill
    \begin{subfigure}[b]{0.24\textwidth}
        \centering
        \includegraphics[width=\textwidth]{figs/test_v3_eval_lr5e-1_4_loss_curve.pdf}
        \caption{3 directions}
        \label{fig:v3}
    \end{subfigure}
    \hfill
    \begin{subfigure}[b]{0.24\textwidth}
        \centering
        \includegraphics[width=\textwidth]{figs/test_v5_eval_lr5e-2_4_loss_curve.pdf}
        \caption{5 directions}
        \label{fig:v5}
    \end{subfigure}
    \hfill
    \begin{subfigure}[b]{0.24\textwidth}
        \centering
        \includegraphics[width=\textwidth]{figs/test_v300_eval_lr5e-2_4_loss_curve.pdf}
        \caption{300 directions}
        \label{fig:v300}
    \end{subfigure}
    
    \caption{Different direction number loss curve.}
    \label{fig:direction}
\end{figure}
\begin{figure}[h]
    \centering
    
    \begin{subfigure}[b]{0.24\textwidth}
        \centering
        \includegraphics[width=\textwidth]{figs/test_fg_v1_lr5e-1_4_loss_curve.pdf}
        \caption{1 direction}
        \label{fig:v1_cos}
    \end{subfigure}
    \hfill
    \begin{subfigure}[b]{0.24\textwidth}
        \centering
        \includegraphics[width=\textwidth]{figs/test_fg_v3_lr5e-1_4_loss_curve.pdf}
        \caption{3 directions}
        \label{fig:v3_cos}
    \end{subfigure}
    \hfill
    \begin{subfigure}[b]{0.24\textwidth}
        \centering
        \includegraphics[width=\textwidth]{figs/test_fg_v5_lr5e-2_4_loss_curve.pdf}
        \caption{5 directions}
        \label{fig:v5_cos}
    \end{subfigure}
    \hfill
    \begin{subfigure}[b]{0.24\textwidth}
        \centering
        \includegraphics[width=\textwidth]{figs/test_fg_v300_lr5e-2_4_loss_curve.pdf}
        \caption{300 directions}
        \label{fig:v300_cos}
    \end{subfigure}
    
    \caption{Different direction number loss curve without Cosine Annealing Learning Rate.}
    \label{fig:cos_lr}
\end{figure}
We explore the hyperparameters for \sys.
Figure~\ref{fig:direction} and Figure~\ref{fig:cos_lr} analyze the interaction between the number of sampled directions and learning rate schedules in knowledge editing. While prior work on knowledge editing and zeroth-order optimization primarily employed static learning rates, as shown in Figure~\ref{fig:direction}, our experiments highlight the significant advantage of cosine annealing, demonstrated in Figure~\ref{fig:cos_lr}. With a static learning rate, effective parameter updates require at least 300 sampled directions, and optimization completely fails with only 1–5 directions due to persistent loss plateaus. In contrast, cosine annealing achieves noticeable loss reduction with just one sampled direction and delivers practical editing performance with only five directions—a 60$\times$ improvement in sampling efficiency. This empirically confirms that adaptive learning rate scheduling inherently reduces gradient estimation noise in zeroth-order optimization, which is especially critical in low-sample regimes where static learning rates face inherent limitations.

% We provide the complete hyperparameter configurations used in our experiments in Table~\ref{tab:hparams}.
% \input{figs/hypersetting}

\section{Examples of Personal Information Injection on Mobile}
Table~\ref{tab:examples} shows how models memorize personalized information through simple conversations. In the first example (e.g., "My address is No.1010, Beijing Road"), the user provide specific information. When asked later ("What is my address?"), the edited model responds accurately—correctly recalling exact numbers, names like "Red Star Primary School," and even adjusting text cases (e.g., "reading" → "Reading"). Without such edits, the model often returns incorrect answers, including random symbols (e.g., ., , ,) or unrelated content. The model also reliably associates related terms, such as identifying that “dad” corresponds to “father” across different conversations.
\begin{table*}[t!]
% \centering
\vspace{-200pt}
\small
\begin{tabular}{p{2.5cm} p{11cm}}
\toprule
\textbf{Scenario} & \textbf{Dialogue Flow} \\
\midrule
\multirow{4}{*}{Address} 
& \textbf{First chat:} \\
& \quad usr: My address is \textcolor{blue}{No.1010, Beijing Road} \\
& \textbf{Second chat:} \\
& \quad usr: What is my address? \\
& \quad \textit{Before editing} \\
& \quad model: .,,, \\
& \quad \textit{After editing} \\
& \quad model: \textcolor{blue}{No.1010, Beijing Road} \\
\midrule

\multirow{4}{*}{Daughter's School}
& \textbf{First chat:} \\
& \quad usr: My daughter studies at \textcolor{blue}{Red Star Primary School} \\
& \textbf{Second chat:} \\
& \quad usr: Where my daughter studies at? \\
& \quad \textit{Before editing} \\
& \quad model: thelands Academy School \\
& \quad \textit{After editing} \\
& \quad model: \textcolor{blue}{Red Star Primary School} \\
\midrule

\multirow{4}{*}{Father's Phone}
& \textbf{First chat:} \\
& \quad usr: My father's phone number is \textcolor{blue}{139********} \\
& \textbf{Second chat:} \\
& \quad usr: Please tell me my dad's contact number \\
& \quad \textit{Before editing} \\
& \quad model: 1 521 \\
& \quad \textit{After editing} \\
& \quad model: \textcolor{blue}{139********} \\
\midrule

\multirow{4}{*}{Mother's Hobby}
& \textbf{First chat:} \\
& \quad usr: My mother's favorite hobby is \textcolor{blue}{reading} \\
& \textbf{Second chat:} \\
& \quad usr: What does my mom like to do? \\
& \quad \textit{Before editing} \\ 
& \quad model: to \\
& \quad \textit{After editing} \\
& \quad model: \textcolor{blue}{Reading} \\
\bottomrule
\end{tabular}
\caption{\sys examples. Each block demonstrates a edit example; model outputs before and after editing are shown.}
\label{tab:examples}
\end{table*}
